# Supplementary material for: Adversarial Generation of Continuous Images
Source: arXiv:2011.12026 source file (2021-06-28)
Supplement: Supplementary file 2 [file training-on-top-of-weights.tex]

\section{Training $\D$ on top of INR weights}\label{ap:training-D-on-top-of-weights}
In theory, one can train $\D$ on top of $\F$ weights since conversion of an ImageNet-sized dataset of images into a dataset of INRs can be done in several days, depending on the $\F$ architecture.
But such an approach has 3 severe downsides: 1) changing INR architecture would require re-converting the whole dataset severely restricting preliminary experimentation; 2) input size for $D$ inreases a lot 3) one inevitably loses information during the conversion process (INR reconstruction may not be perfect).
That's why we opt for training $D$ on top of real images.
We do this by evaluating $F_{\bm\theta}(\bm p)$ on each iteration at each pixel coordinate of $H \times W$ grid.
Our efficient INR implementation via batch matrix multiplication allows to make this process $\times 2$ times faster compared to an inference process of a traditional convolutional GAN of comparable size.
